# Supplementary material for: Convergence Analysis of Proximal Gradient with Momentum for Nonconvex Optimization
Source: arXiv:1705.04925 source file (2017-05-14)
Supplement: Supplementary file 1 [file appendix.tex]

%!TEX root = paper.tex
\appendix
\section{Proof of \Cref{thm: limit_point}}\label{append: limit}
We first recall the following lemma.
\begin{lemma}[Lemma 1, Gong 2013]\label{lemma: descent}
Under \Cref{assum:func}.\{3\}. For any $\eta >0$ and any $\xb, \yb \in \RR^d$ such that $\xb = \prox{\eta g} (\yb - \eta \nabla f(\yb))$, one has that
	\begin{align*}
		F(\xb) \le F(\yb)- (\tfrac{1}{2{\eta}} - \tfrac{L}{2}) \|\xb-\yb\|^2.
	\end{align*}
\end{lemma}

Applying \Cref{lemma: descent} with $\xb = \xb_k, \yb = \yb_k$, we obtain that
\begin{align}\label{eq: decrease}
F(\xb_k) \le F(\yb_k)- (\tfrac{1}{2{\eta}} - \tfrac{L}{2}) \|\xb_k-\yb_k\|^2.
\end{align}
Since $\eta< \frac{1}{L}$, it follows that $F(\xb_k) \le F(\yb_k)$. Moreover, the update rule of APGnc guarantees that $F(\yb_{k+1}) \le F(\xb_k)$. In summary, for all $k$ the following inequality holds:
\begin{align}\label{eq: descent}
F(\yb_{k+1}) \le F (\xb_k)\le F(\yb_k) \le F(\xb_{k-1}).
\end{align}
Combing further with the fact that $F(\xb_k), F(\yb_k) \ge \inf F>-\infty$ for all $k$, we conclude that $\{F(\xb_k)\}, \{F(\yb_k)\}$ converge to the same limit $F^*$, \ie,
\begin{align}\label{eq: func_limit}
\lim_{k\to \infty} F(\xb_k) = \lim_{k\to \infty} F(\yb_k) = F^*.
\end{align}
On the other hand, by induction we conclude from \cref{eq: descent} that for all $k$
\[
F(\yb_{k})\le F(\xb_0), \quad F(\xb_{k})\le F(\xb_0).
\]
Combining with \Cref{assum:func}.1 that $F$ has bounded sublevel set, we conclude that $\{\xb_k\}$ and $\{\yb_{k}\}$ are bounded and thus have bounded limit points.
Now combining \cref{eq: decrease} and \cref{eq: descent} yields
\begin{align}
(\tfrac{1}{2{\eta}}-\tfrac{L}{2})\|\yb_{k}-\xb_k\|^2 &\le F(\yb_k)-F(\xb_k) \nonumber \\
&\le F(\yb_k)-F(\yb_{k+1}),
\end{align}
which, after telescoping over $k$ and letting $k\to \infty$, becomes
\begin{align}
\sum_{k=1}^\infty (\tfrac{1}{2{\eta}}-\tfrac{L}{2})\|\yb_{k}-\xb_k\|^2 \le F(\yb_1)-\inf F <\infty.
\end{align}
This further implies that $\|\yb_{k}-\xb_k\| \to 0$, and hence $\{\xb_k\}$ and $\{\yb_{k}\}$ share the same set of limit points $\Omega$. Note that $\Omega$ is closed (it is a set of limit points) and bounded, we conclude that $\Omega$ is compact in $\RR^d$.

By optimality condition of the proximal gradient step of APGnc, we obtain that
\begin{align}
	-\nabla f(\yb_k)- \tfrac{1}{{\eta}}(\xb_k-\yb_k) &\in \partial g(\xb_k)  \nonumber\\
 	\Leftrightarrow  \underbrace{\nabla f(\xb_{k})-\nabla f(\yb_k)-\tfrac{1}{{\eta}}(\xb_k-\yb_k)}_{\ub_k} &\in \partial F(\xb_k), \label{ast}
\end{align}
which further implies that
\begin{align}
	\|\ub_k\| &= \|\nabla f(\xb_{k})-\nabla f(\yb_k)-\tfrac{1}{{\eta}}(\xb_k-\yb_k)\| \nonumber\\
	&\le (L+\tfrac{1}{{\eta}}) \|\yb_{k}-\xb_k\| \to 0.   \label{eq: u_k}
\end{align}
Consider any limit point $\zb' \in \Omega$, and w.l.o.g we write $\xb_k \to \zb', ~\yb_k \to \zb'$ by restricting to a subsequence. By the definition of the proximal map, the proximal gradient step of APGnc implies that
\begin{align}
&\inner{\nabla f(\yb_{k})}{\xb_{k}-\yb_{k}} +\tfrac{1}{2{\eta}}\|\yb_{k}-\xb_{k}\|^2+g(\xb_{k}) \nonumber\\
&\quad \le \inner{\nabla f(\yb_{k})}{\zb'-\yb_{k}} + \tfrac{1}{2{\eta}}\|\zb'-\yb_{k}\|^2+g(\zb').
\end{align}
Taking $\limsup$ on both sides and note that $\xb_{k}-\yb_{k} \to 0, ~\yb_k \to \zb'$, we obtain that $\limsup_{k\to \infty} g(\xb_{k}) \le g(\zb').$
Since $g$ is lower semicontinuous and $\xb_k \to \zb'$, it follows that $\limsup_{k\to \infty} g(\xb_{k}) \ge g(\zb')$.
Combining both inequalities, we conclude that $\lim_{k\to \infty} g(\xb_{k}) = g(\zb').$
Note that the continuity of $f$ yields $\lim_{k\to \infty}  f(\xb_{k}) = f(\zb'),$ we then conclude that $\lim_{k\to \infty}  F(\xb_{k}) = F(\zb')$. Since $\lim_{k\to \infty} F(\xb_k) = F^*$ by \cref{eq: func_limit}, we conclude that
\begin{align}
	F(\zb') \equiv F^*, \quad \forall \zb' \in  \Omega.
\end{align}
Hence, $F$ remains constant on the compact set $\Omega$.
To this end, we have established $\xb_k \to \zb', ~F(\xb_k) \to F(\zb')$ and that $\partial F(\xb_k) \ni \ub_k \to 0$. Recall the definition of limiting sub-differential, we conclude that $0\in \partial F(\zb')$ for all $\zb' \in \Omega$.

\section{Proof of \Cref{thm: KL_rate}}
Throughout the proof we assume that $F(\xb_k) \ne F^*$ for all $k$ because otherwise the algorithm terminates and the conclusions hold trivially. We also denote $k_0$ as a sufficiently large positive integer.

Combining \cref{eq: decrease} and \cref{eq: descent} yields that
\begin{align}
	F(\xb_{k+1}) \le F(\xb_{k})-(\tfrac{1}{2{\eta}} - \tfrac{L}{2})\|\yb_{k+1}-\xb_{k+1}\|^2. \label{eq: func_bound}
\end{align}
Moreover, \cref{ast} and \cref{eq: u_k} imply that
\begin{align}
\dist_{\partial F (\xb_k)} (\mathbf{0}) \le (L+\tfrac{1}{{\eta}}) \|\yb_{k}-\xb_k\|. \label{eq: subdiff_bound}
\end{align}
We have shown in \Cref{append: limit} that $F(\xb_k) \downarrow F^*$, and it is also clear that $\dist_{\Omega}(\xb_k) \to 0$. Thus, for any $\epsilon, \delta>0$ and all $k\ge k_0$, we have
\[
\xb_k\in \{\xb~|~ \dist_{\Omega}(\xb) \le \epsilon,  F^*<F(\xb)<F^*+\delta\}.
\]
Since $\Omega$ is compact and $F$ is constant on it,  the uniformized KL property implies that for all $k\ge k_0$
\begin{align}
\varphi' (F(\xb_k)-F^*)\dist_{\partial F(\xb_k)}(\mathbf{0})\ge 1. \label{eq: uni_KL}
\end{align}
Recall that $r_k:=F(\xb_k)-F^*$. Then \cref{eq: uni_KL} is equivalent to
\begin{align*}
1&\le \left(\varphi^\prime \left(r_k\right)\dist_{\partial F\left(\xb_k\right)}\left(\mathbf{0} \right)\right)^2\\
& \overset{(i)}{\le} \left(\varphi^\prime\left(r_k\right)\right)^2\left(\tfrac{1}{{\eta}}+L\right)^2\|\yb_k-\xb_{k}\|^2\\
& \overset{(ii)}{\le}  \left(\varphi^\prime\left(r_k\right)\right)^2 \tfrac{\left(\tfrac{1}{{\eta}}+L\right)^2}{\frac{1}{2{\eta}}-\frac{L}{2}}[F\left(\xb_{k-1}\right)-F\left(\xb_k\right)]\\
&\le d_1  \left(\varphi^\prime\left(r_k\right)\right)^2 \left(r_{k-1}-r_k\right),
\end{align*}
 where (i) is due to \cref{eq: subdiff_bound}, (ii) follows from \cref{eq: func_bound}, and $d_1=\left(\frac{1}{{\eta}}+L\right)^2/\left(\frac{1}{2{\eta}}-\frac{L}{2}\right)$.
Since $\varphi \left(t\right)=\frac{c}{\theta}t^\theta$, we have that $\varphi^\prime\left(t\right)=ct^{\theta-1}$. Thus the above inequality becomes
\begin{align}
1\le d_1c^2r_k^{2\theta-2}\left(r_{k-1}-r_k\right). \label{eq: func_rate}
\end{align}
It has been shown in \cite{Lihuan_2015,Frankel2015} that sequence $\{r_k\}$ satisfying the above inductive property converges to zero at different rates according to $\theta$ as stated in the theorem.

\section{Proof of \Cref{thm: APGnc_inexact}}
\textbf{$g$ non-convex, $\epsilon_k=0$}: In this setting, we first prove the following inexact version of \Cref{lemma: descent}.
\begin{lemma}\label{lemma: descent_inex}
	Under \Cref{assum:func}.3. For any $\eta >0$ and any $\xb, \yb \in \RR^d$ such that $\xb = \prox{\eta g} (\yb - \eta (\nabla f(\yb) + \eb))$, one has that
	\begin{align*}
	F(\xb) \le F(\yb) + (\tfrac{L}{2} - \tfrac{1}{2\eta})\|\xb - \yb\|^2 + \|\xb - \yb\|\|\eb\|.
	\end{align*}
\end{lemma}
\begin{proof}
	By \Cref{assum:func}.3 we have that
\[
f(\xb) \le f(\yb) + \inner{\xb - \yb}{\nabla f(\yb)} + \tfrac{L}{2}\|\xb - \yb\|^2.
\]
Also, by the definition of proximal map, the proximal gradient step implies that
\[
g(\xb) + \tfrac{1}{2\eta} \|\xb - \yb + \eta(\nabla f(\yb) + \eb)\|^2 \le g(\yb) + \tfrac{1}{2\eta} \|\eta(\nabla f(\yb) + \eb)\|^2,
\]
which, after simplifications becomes that
\[
g(\xb)  \le g(\yb) - \tfrac{1}{2\eta} \|\xb - \yb\|^2 - \inner{\xb-\yb}{(\nabla f(\yb) + \eb)}.
\]
Combine the above two inequalities further gives that
\[
F(\xb) \le F(\yb) + (\tfrac{L}{2} - \tfrac{1}{2\eta})\|\xb - \yb\|^2 + \|\xb - \yb\|\|\eb\|.
\]
\end{proof}

Using \Cref{lemma: descent_inex} with $\xb = \xb_k, \yb = \yb_k, \eb = \eb_k$ and notice the fact that $\|\eb_k\| \le \gamma\|\xb_k - \yb_k\|$, we obtain that
\begin{align}
	F(\xb_k) \le F(\yb_k) + (\gamma + \tfrac{L}{2} - \tfrac{1}{2\eta})\|\xb_k - \yb_k\|^2. \label{eq: suff_inexact}
\end{align}
Moreover, the optimality condition of the proximal gradient step with gradient error gives that
By optimality condition of the proximal gradient step of APGnc, we obtain that
\begin{align*}
 \nabla f(\xb_{k})-\nabla f(\yb_k)-\eb_k-\tfrac{1}{{\eta}}(\xb_k-\yb_k) &\in \partial F(\xb_k),
\end{align*}
which further implies that
\begin{align}
\dist_{\partial F (\xb_k)} (\mathbf{0}) \le (\gamma+L+\tfrac{1}{{\eta}}) \|\yb_{k}-\xb_k\|. \label{eq: subdiff_bound_inexact}
\end{align}
Notice that \cref{eq: suff_inexact} and \cref{eq: subdiff_bound_inexact} are parallel to the key inequalities \cref{eq: func_bound} and \cref{eq: subdiff_bound} in the analysis of exact APGnc. Thus, by choosing $\eta < \frac{1}{2\gamma + L}$ and redefining $d_1 = (\frac{1}{\eta} + L + \gamma)^2 / (\frac{1}{2\eta} - \frac{L}{2} - \gamma)$, all the statements in \Cref{thm: limit_point} remain true and the convergence rates in \Cref{thm: KL_rate} remain the same order with a worse constant.

\textbf{$g$ convex}:
We first present the following lemma.
\begin{lemma}\label{eq: subdiff_epsilon}
For any $\xb, \vb \in \RR^d$, let $\ub' \in \partial_{\epsilon} g(\xb)$ such that $\nabla f(\xb) + \ub'$ has minimal norm. Denote $\xi := \dist_{\partial g(\xb)} (\ub')$, then we have
\begin{align}
	\dist_{\partial F(\xb)} (\zero) \le  \dist_{\nabla f(\xb) + \partial_{\epsilon} g(\xb)} (\zero) + \xi.
\end{align}
\end{lemma}
\begin{proof}
	We observe the following
	\begin{align}
		\dist_{\partial F(\xb)} (\zero) &= \min_{\ub \in \partial g(\xb)} \|\nabla f(\xb) + \ub\| \nonumber\\
		&=  \min_{\ub \in \partial g(\xb)} \|\nabla f(\xb) + \ub' + \ub - \ub'\|, ~\forall \ub' \in \partial_{\epsilon} g(\xb) \nonumber\\
		&\le  \|\nabla f(\xb) + \ub'\| + \min_{\ub \in \partial g(\xb)} \|\ub - \ub'\|, ~\forall \ub' \in \partial_{\epsilon} g(\xb) \nonumber\\
		&\le \min_{\ub' \in \partial_{\epsilon}} g(\xb) \|\nabla f(\xb) + \ub'\| + \xi \nonumber\\
	&=  \dist_{\nabla f(\xb) + \partial_{\epsilon} g(\xb)} (\zero) + \xi.
	\end{align}
\end{proof}

Recall that we have two inexactness, \ie, $\xb_k = \prox{\eta g}^{\epsilon_k} (\yb_k - \eta (\nabla f(\yb_k) + \eb_k))$. Following a proof similar to that of \Cref{lemma: descent_inex} and notice that $\epsilon_k \le \delta\|\xb_k - \yb_k\|^2$, we can obtain that
\begin{align}
F(\xb_k) &\le F(\yb_k) + (\gamma + \tfrac{L}{2} - \tfrac{1}{2\eta})\|\xb_k - \yb_k\|^2 + \epsilon_k \nonumber\\
&\le F(\yb_k) + (\gamma' + \tfrac{L}{2} - \tfrac{1}{2\eta})\|\xb_k - \yb_k\|^2 \label{eq: suff_inexact2}
\end{align}
for some $\gamma' > \gamma >0$.
Since $g$ is convex, by Lemma 2 in \cite{inexact_pga} one can exhibit $\vb_k$ with $\|\vb_k\|\le \sqrt{2\eta\epsilon_k}$ such that
\[
\tfrac{1}{\eta}[\yb_k - \xb_k - \eta (\nabla f(\yb_k) + \eb_k) - \vb_k] \in \partial_{\epsilon_k} g(\xb_k).
\]
This implies that
\[
\dist_{\nabla f(\xb_k)+\partial_{\epsilon_k} g(\xb_k)}(\zero) \le (\gamma + \tfrac{1}{\eta} + L)\|\xb_k - \yb_k\| + \sqrt{\tfrac{2\epsilon_k}{\eta}}.
\]
Apply \Cref{eq: subdiff_epsilon} and notice that $\epsilon_k \le \delta\|\xb_k - \yb_k\|^2, \xi_k \le \lambda\|\xb_k - \yb_k\|$, we obtain that
\begin{align}
	\dist_{\partial F(\xb_k)}(\zero) \le (\gamma' + \frac{1}{\eta} + L)\|\xb_k - \yb_k\|\label{eq: subdiff_2}
\end{align}
for some $\gamma'>\gamma>0$. Now \cref{eq: suff_inexact2} and \cref{eq: subdiff_2} are parallel to the key inequalities \cref{eq: func_bound} and \cref{eq: subdiff_bound} in the analysis of exact APGnc. Thus, by choosing $\eta < \frac{1}{2\gamma' + L}$ and redefining $d_1 = (\frac{1}{\eta} + L + \gamma')^2 / (\frac{1}{2\eta} - \frac{L}{2} - \gamma')$, all the statements in \Cref{thm: limit_point} remain true and the convergence rates in \Cref{thm: KL_rate} remain the same order with a worse constant.

\section{Proof of \Cref{thm: svrg}}\label{sec: thm: svrg}
We first define the following quantities for the convenience of the proof.
\begin{align}
&c_{t}=c_{t+1}(1+\tfrac{1}{m})+\tfrac{\eta L^2}{2},\ \ c_m=0,\label{eq: c_t}\\
&R_k^{t} \coloneqq \Ebb\left[F(\xb_k^{t})+c_t\|\xb_k^{t}-\xb_k^0\|^2\right], \\
&\bar{\xb}^{t+1}_k=\prox{\eta g}(\xb^t_k-\eta\nabla f(\xb^t_k)).\label{eq: ref}
\end{align}
	Note that $\bar{\xb}_k^{t+1}$ is a reference sequence introduced for the convenience of analysis, and is not being computed in the implementation of the algorithm.
	Then it has been shown in the proof of Theorem 5 of \cite{NIPS2016_6116} that
	\begin{align}\label{reddi}
	R_k^{t+1} \le R_k^t+\left(L-\tfrac{1}{2\eta}\right)\Ebb\left[\|\bar{\xb}_k^{t+1}-{\xb}_k^t\|^2\right].
	\end{align}

	Telescoping \cref{reddi} over $t$ from $t=1$ to $t=m-1$, we obtain
	\begin{align}
	\Ebb[F(\xb_k^{m})] \le \Ebb\left[F(\bar{\xb}_k^1)+c_1\|\bar{\xb}^1_k-\xb_k^0\|^2+\sum\limits_{t=1}^{m-1}\left(L-\tfrac{1}{2\eta}\right)\|\bar{\xb}_k^{t+1}-{\xb}_k^t\|^2\right]. \label{eq: reddi_tele}
	\end{align}
Following from \cref{eq: c_t}, a simple induction shows that $c_t\le \eta L^2m$. Setting $\eta < \frac{1}{2L}$ and recalling that $F(\yb_k)\le F(\xb_{k-1}^m)$.,  \cref{eq: reddi_tele} further implies that
	\begin{align}\label{c1}
	\Ebb[F(\yb_{k+1})]\le	\Ebb[F(\xb_k^{m})] \le \Ebb[F(\bar{\xb}^1_k)]+\eta L^2m\Ebb[\|\bar{\xb}^1_k-\xb^0_k\|^2].
	\end{align}
	Now telescoping \cref{reddi} again over $t$ from $t=0$ to $t=m-1$ and applying \cref{c1}, we obtain
	\begin{align}\label{nonincreasing}
	\Ebb[F(\xb^{m}_k)]\le \Ebb[F(\yb_k)]+\sum\limits^{m-1}_{t=0}(L-\tfrac{1}{2\eta})\Ebb\left[\|\bar{\xb}_k^{t+1}-{\xb}_k^t\|^2\right].
	\end{align}
	Combining all the above facts, we conclude that for $\eta < \frac{1}{2L}$
	\begin{align}
	\Ebb[F(\yb_k)] \le \Ebb[F(\yb_{k-1})]\le \ldots \le F(\yb_{0}).
	\end{align}

	Since $\Ebb [F(\cdot)]$ is bounded below, $\Ebb[ F(\yb_k)]$ decreases to a finite limit, say, $F^*$. Define $r_k=\Ebb\left[ F(\yb_k)-F^\ast\right] $, and assume $r_k >0$ for all $k$ (since otherwise $r_k = 0$ and the algorithm terminates). Applying the \KL property with $\theta=1/2$, we obtain
	\begin{align}
	\tfrac{1}{c} (F(\xb)-F^\ast)^{\frac{1}{2}} \le \dist_{\partial F(\xb)} (\zero).
	\end{align}
	Setting $\xb=\bar{\xb}_k^1$, we further obtain
	\begin{align}
	\tfrac{1}{c^2} (F(\bar{\xb}_k^1)-F^\ast) \le \dist_{\partial F(\bar{\xb}^1_k)}^2 (\zero) \le \left(L+\tfrac{1}{\eta}\right)^2\|\bar{\xb}^1_k-\yb_k\|^2,
	\end{align}
	where the last inequality is due to \cref{eq: ref}.
	Taking expectation over both sides and using \cref{c1}, we obtain
	\begin{align}
	\tfrac{1}{c^2}	\Ebb[F(\xb_k^m)-F^\ast]-\tfrac{\eta L^2 m}{c^2}\Ebb\left[\|\bar{\xb}_k^1-\xb_k^0\|^2\right] \le  \left(L+\tfrac{1}{\eta}\right)^2\Ebb\left[\|\bar{\xb}^1_k-\yb_k\|^2\right].
	\end{align}
	Noting that $\xb_k^0=\yb_k$ and $\Ebb F(\yb_{k+1})	\le	\Ebb F(\xb_k^m)$, we then rearrange the above inequality and obtain
	\begin{align}
	\tfrac{1}{c^2}	\Ebb[F(\yb_{k+1})-F^\ast]	\le	\tfrac{1}{c^2}	\Ebb[F(\xb_k^m)-F^\ast] &\le \left[\left(L+\tfrac{1}{\eta}\right)^2+\tfrac{\eta L^2 m}{c^2}\right]\Ebb\left[\|\bar{\xb}^1_k-\yb_k\|^2\right]\\
	&\le \tfrac{\left(L+\frac{1}{\eta}\right)^2+\frac{\eta L^2 m}{c^2}}{\frac{1}{2\eta}-L}\left(\Ebb[F(\yb_k)]-E[F(\yb_{k+1})]\right) ,
	\end{align}
	which can be further rewritten as
	\begin{align}
	r_{k+1} \le d \left(r_k-r_{k+1}\right), 
	\end{align}
where $d=\tfrac{c^2\left(L+\frac{1}{\eta}\right)^2+{\eta L^2 m}}{\frac{1}{2\eta}-L}$. Then a simple induction yields that
	\begin{align}
	r_{k+1} \le \left(\tfrac{d}{d+1}\right)^{k+1}\left(F(\yb_0)-F^\ast\right).
	\end{align} 
\section{Proof of \Cref{thm: svrg_inexact}}
We first introduce some auxiliary lemmas.
	\begin{lemma}\label{lemma1}
		Consider the convex function $g$ and $\xb,\yb \in \RR^d$ such that $\yb=\prox{\eta g}^\epsilon (\xb)$ for some $\epsilon >0$. Then, there exists $\|\ib\| \le \sqrt{2\eta \epsilon}$ that satisfies the following inequality for all $\zb\in \RR^d$.
		\begin{align}
		g(\yb)+\tfrac{1}{2\eta}\|\yb-\xb\|^2 \le g(\zb)+\tfrac{1}{2\eta}\|\zb-\xb\|^2-\tfrac{1}{2\eta}\|\yb-\zb\|^2+\langle \yb-\zb,\tfrac{1}{\eta}\ib \rangle		+\epsilon.	
		\end{align}
	\end{lemma}
	\begin{proof}
		By Lemma 2 in \cite{inexact_pga}, there exists $\|\ib\| \le \sqrt{2\eta \epsilon}$ such that
		\begin{align}
		\tfrac{1}{\eta}\left(\xb-\yb-\ib\right) \in \partial_\epsilon g(\yb).
		\end{align}
		Then, the definition of $\epsilon$-subdifferential implies that
		\begin{align}
		g(\zb)-g(\yb) &\ge \langle \zb-\yb, \partial_\epsilon g(\yb)\rangle-\epsilon = \langle \zb-\yb, \tfrac{1}{\eta}\left(\xb-\yb-\ib\right)\rangle-\epsilon,~\forall~\zb \in \RR^d.
		\end{align}
		The desired result follows by rearranging the above inequality.
	\end{proof}
	\begin{lemma}\label{lemma2}
		Consider the convex function $g$ and $\xb,\yb, \db\in \RR^d$ such that $\yb=\prox{\eta g}^\epsilon(\xb-\eta \db)$ for some $\epsilon >0$. Then, there exists $\|\ib\| \le \sqrt{2\eta \epsilon}$ that satisfies the following inequality for all $\zb\in \RR^d$.
		\begin{align}
		g(\yb)=\langle \yb-\zb, \db -\tfrac{1}{\eta} \ib\rangle \le g(\zb)+ \tfrac{1}{2\eta} \left[\|\zb-\xb\|^2-\|\yb-\zb\|^2-\|\yb-\xb\|^2\right]+\epsilon.
		\end{align}
	\end{lemma}
	\begin{proof}
		By \Cref{lemma1}, we obtain the following inequality for all $\zb\in \RR^d$.
		\begin{align}
g(\yb) &+\langle \yb-\xb,\db\rangle +\tfrac{1}{2\eta}\|\yb-\xb\|^2+\frac{\eta}{2}\|\db\|^2 \nonumber \\
& \quad \le g(\zb)+\tfrac{1}{2\eta}\|\zb-\xb+\eta \db\|^2-\tfrac{1}{2\eta}\|\yb-\zb\|^2+\langle \yb-\zb,\tfrac{1}{\eta} \ib\rangle+\epsilon \nonumber \\
		&\quad = g(\zb)+\langle \zb-\xb, \db\rangle \tfrac{1}{2\eta}\|\zb-\xb\|^2+\tfrac{\eta}{2}\|\db\|^2-\tfrac{1}{2\eta}\|\yb-\zb\|^2+\langle \yb-\zb,\tfrac{1}{\eta} \ib \rangle+\epsilon.
		\end{align}
		The desired result follows by rearranging the above inequality.
	\end{proof}
	\begin{lemma}\label{lemma3}
		Consider the convex function $g$ and $\xb,\yb, \db\in \RR^d$ such that $\yb=\prox{\eta g}^\epsilon(\xb-\eta \db)$ for some $\epsilon >0$. Then, there exists $\|\ib\| \le \sqrt{2\eta \epsilon}$ that satisfies the following inequality for all $\zb\in \RR^d$.
		\begin{align}
		F(\yb)+\langle \yb-\zb,\db-\tfrac{1}{\eta} \ib-\nabla f(\xb) \rangle \le F(\zb)+\left(\tfrac{L}{2}-\tfrac{1}{2\eta}\right)\|\yb-\xb\|^2+\left(\tfrac{L}{2}+\tfrac{1}{2\eta}\right)\|\zb-\xb\|^2-\tfrac{1}{2\eta}\|\yb-\zb\|^2+\epsilon.
		\end{align}
		\begin{proof}
			By Lipschitz continuity of $\nabla f$, we obtain
			\begin{align}
			f(\yb) \le f(\xb)+\langle \nabla f(\xb),\yb-\xb \rangle +\tfrac{L}{2}\|\yb-\xb\|^2,\\
			f(\xb) \le f(\zb)+\langle \nabla f(\xb),\xb-\zb \rangle +\tfrac{L}{2}\|\xb-\zb\|^2.
			\end{align}
			Adding the above inequalities together yields
			\begin{align}
			f(\yb)\le f(\zb)+\langle \nabla f(\xb), \yb-\zb \rangle +\tfrac{L}{2}\left[\|\yb-\xb\|^2+\|\zb-\xb\|^2\right].
			\end{align}
			Combining with \Cref{lemma2}, we then obtain the desired result.
		\end{proof}
	\end{lemma}
	
	Recall the reference sequence $\bar{\xb}^{t+1}_k=\prox{\eta g}(\xb^t_k-\eta\nabla f(\xb^t_k))$.	
	Applying \Cref{lemma3} with $\epsilon=0$, $\yb=\bar{\xb}^{t+1}_k$, $\zb=\xb^t_k$, and $\db=\nabla f(\xb^t_k)$ and taking expectation on both sides, we obtain
	\begin{align}\label{24}
	\Ebb[F(\bar{\xb}^{t+1}_k)] \le \Ebb\left[F(\xb^t_k)+\left(\tfrac{L}{2}-\tfrac{1}{2\eta}\right)\|\bar{\xb}^{t+1}_k) - \xb^t_k\|^2-\tfrac{1}{2\eta}\|\bar{\xb}^{t+1}_k - \xb^t_k\|^2\right].
	\end{align}
	Similarly, applying \Cref{lemma3} with $\epsilon=\epsilon_k^t$, $\yb=\xb^{t+1}_{k}$, $\zb=\bar\xb^{t+1}_k$, $\db=\vb_k^t$ and taking expectation on both sides, we obtain
	\begin{align}\label{25}
	\Ebb[F({\xb}^{t+1}_k)] &\le \Ebb\left[F(\bar\xb^{t+1}_k)+\langle\xb^{t+1}_k-\bar{\xb}^{t+1}_k, \nabla f\left(\xb^t_k \right)-\vb_k^t+\tfrac{1}{\eta}\ib_k \rangle\right.\nonumber\\
	&\left.+\left(\tfrac{L}{2}-\tfrac{1}{2\eta}\right)\|{\xb}^{t+1}_k - \xb^t_k\|^2+\left(\tfrac{L}{2}+\tfrac{1}{2\eta}\right)\|\bar{\xb}^{t+1}_k - \xb^t_k\|^2-\tfrac{1}{2\eta}\|\bar{\xb}^{t+1}_k - \xb^{t+1}_k\|^2+\epsilon_k^t\right].
	\end{align}
	Adding \cref{24} and \cref{25} together yields
	\begin{align}\label{26}
	\Ebb[F({\xb}^{t+1}_k)] \le \Ebb\left[F(\xb^t_k)+\left({L}-\tfrac{1}{2\eta}\right)\|\bar{\xb}^{t+1}_k- \xb^t_k\|^2 +\left(\tfrac{L}{2}-\tfrac{1}{2\eta}\right)\|{\xb}^{t+1}_k - \xb^t_k\|^2-\tfrac{1}{2\eta}\|\bar{\xb}^{t+1}_k - \xb^{t+1}_k\|^2+T\right]
	\end{align}
	where $T=\langle\xb^{t+1}_k-\bar{\xb}^{t+1}_k, \nabla f\left(\xb^t_k \right)-\vb_k^t+\frac{\mathbf{i}_k}{\eta} \rangle+\epsilon_k^t$.
	Now we bound $\Ebb[T]$ as follows.
	\begin{align}
	\Ebb[T] &\le \tfrac{1}{2\eta} \Ebb\left[ \|\xb^{t+1}_k -  \xb^{t+1}_k \|^2\right]+\tfrac{\eta}{2}\Ebb\left[ \| \nabla f\left(\xb^t_k \right)-\vb_k^t+\tfrac{\mathbf{i}_k}{\eta}\|^2 \right] +\epsilon_k^t \\
	&\le 	\tfrac{1}{2\eta} \Ebb\left[ \|\xb^{t+1}_k -  \xb^{t+1}_k \|^2\right]+{\eta}\Ebb\left[ \| \nabla f\left(\xb^t_k \right)-\vb_k^t\|^2 \right] +\eta \Ebb\left[ \|\tfrac{\mathbf{i}_k}{\eta} \|^2\right]+\epsilon_k^t \\
	&\le \tfrac{1}{2\eta} \Ebb\left[ \|\xb^{t+1}_k -  \xb^{t+1}_k \|^2\right]+{\eta}\Ebb\left[ \| \nabla f\left(\xb^t_k \right)-\vb_k^t\|^2 \right] +3\epsilon_k^t.
	\end{align}
	By Lemma 3 of \cite{NIPS2016_6116}, it holds that $\Ebb\left[ \| \nabla f\left(\xb^t_k \right)-\vb_k^t\|^2 \right] \le L^2 \Ebb\left[ \|\xb^t_k- \xb^0_{k}\|^2\right].$ Combining with the above inequality,	
	we further obtain that
	\begin{align}
	\Ebb[T]\le \tfrac{1}{2\eta} \Ebb\left[ \|\xb^{t+1}_k -  \xb^{t+1}_k \|^2\right]+\eta L^2 \Ebb\left[ \|\xb^t_k- \xb^0_{k}\|^2\right]+3\epsilon_k^t.
	\end{align}
	Substituting the above result into \cref{26}, we obtain
	\begin{align}
	\Ebb[F({\xb}^{t+1}_k)] \le \Ebb\left[F(\xb^t_k)+\left({L}-\tfrac{1}{2\eta}\right)\|\bar{\xb}^{t+1}_k- \xb^t_k\|^2 +\left(\tfrac{L}{2}-\tfrac{1}{2\eta}\right)\|{\xb}^{t+1}_k - \xb^t_k\|^2+\eta L^2  \|\xb^t_k- \xb^0_{k}\|^2+3\epsilon_k^t\right].
	\end{align}
	Recalling that $R_k^{t} \coloneqq \Ebb\left[F(\xb_k^{t})+c_t\|\xb_k^{t}-\xb_k^0\|^2\right],$ where $	c_t=\eta L^2 \frac{(1+\beta)^{m-t}-1}{\beta}$
	with $\beta>0$.
	Then, we can upper bound $R_k^{t+1}$ as
	\begin{align}
	R_k^{t+1} =& \Ebb \left[ F(\xb^{t+1}_k) +c_{t+1}\|\xb^{t+1}_k-\xb^{t}_k+\xb^{t}_k-\xb^{0}_k\|^2\right]\\
	=&\Ebb \left[ F(\xb^{t+1}_k) +c_{t+1}\left( \|\xb^{t+1}_k-\xb^{t}_k\|^2+\|\xb^{t}_k-\xb^{0}_k\|^2+2\langle\xb^{t+1}_k-\xb^{t}_k,\xb^{t}_k-\xb^{0}_k \rangle\right) \right]\\
	\le & \Ebb\left[ F(\xb^{t+1}_k) +c_{t+1}\left(1+\tfrac{1}{\beta} \right) \|\xb^{t+1}_k-\xb^{t}_k\|^2+c_{t+1}\left(1+{\beta} \right)\|\xb^{t}_k-\xb^{0}_k\|^2  \right]\\
	\le & \Ebb\left[F(\xb^t_k)+\left({L}-\tfrac{1}{2\eta}\right)\|\bar{\xb}^{t+1}_k- \xb^t_k\|^2 +\left[c_{t+1}\left(1+\tfrac{1}{\beta} \right) +\tfrac{L}{2}-\tfrac{1}{2\eta}\right] \|{\xb}^{t+1}_k - \xb^t_k\|^2\right. \\&\left. +\left[ c_{t+1}\left(1+{\beta} \right)+\eta L^2\right]   \|\xb^t_k- \xb^0_{k}\|^2+3\epsilon_k^t\right].
	\end{align}
	
	Setting $\beta=1/m$ in $c_t$ and observe that
	\begin{align}
	c_t=\eta L^2 \tfrac{(1+\beta)^{m-t}-1}{\beta} =\eta L^2m\left( {(1+\beta)^{m-t}-1}\right) \le \eta L^2m\left( e-1\right) \le 2\eta L^2m,
	\end{align}
	which further implies that
	\begin{align}
	c_{t+1}\left(1+\tfrac{1}{\beta} \right)+ \tfrac{L}{2} \le  2\eta L^2m(1+m)\le 4\eta L^2m^2+ \tfrac{L}{2} =4\rho Lm^2+ \tfrac{L}{2} \le \tfrac{1}{2\eta}.
	\end{align}
	
	Also note that $c_t=c_{t+1}(1+\beta)+\eta L^2$. Collecting all these facts, $R_k^{t+1}$ can be further upper bounded by
	\begin{align}\label{reddi+error}
	R_k^{t+1} \le R_k^{t}+\Ebb\left[ \left({L}-\tfrac{1}{2\eta}\right)\|\bar{\xb}^{t+1}_k- \xb^t_k\|^2+3\epsilon_k^t \right].
	\end{align}

	Telescoping \cref{reddi+error} from $t=1$ to $t=m-1$, we obtain
	\begin{align}\label{c1+error}
	\Ebb[F(\xb_k^{m})] \le \Ebb\left[F(\bar{\xb}_k^1)+c_1\|\bar{\xb}^1_k-\xb_k^0\|^2+\sum\limits_{t=1}^{m-1}\left(L-\tfrac{1}{2\eta}\right)\|\bar{\xb}_k^{t+1}-{\xb}_k^t\|^2+\sum\limits_{t=1}^{m-1} 3\epsilon_k^t\right].
	\end{align}
	
	Again, telescoping \cref{reddi+error} from $t=0$ to $t=m-1$ we obtain
	\begin{align}\label{nonincreasing+error}
	\Ebb[F(\yb_{k+1})]\le
	\Ebb[F(\xb^{m}_k)]\le \Ebb[F(\yb_k)]+\sum\limits^{m-1}_{t=0}(L-\tfrac{1}{2\eta})\Ebb\left[\|\bar{\xb}_k^{t+1}-{\xb}_k^t\|^2\right]+3\sum\limits_{t=0}^{m-1}\Ebb\left[  \epsilon_k^t\right].
	\end{align}
	
	Assume $\sum\limits^{m-1}_{t=0}\Ebb\left[\|\bar{\xb}_k^{t+1}-{\xb}_k^t\|^2 \right] >0$, because otherwise the algorithm is terminated. Assume that there exists $\alpha>0$ such that $3\sum\limits_{t=0}^{m-1}\Ebb\left[  \epsilon_k^t\right] \le \alpha \sum\limits^{m-1}_{t=0}\Ebb\left[\|\bar{\xb}_k^{t+1}-{\xb}_k^t\|^2 \right]$ and $\frac{1}{2\eta}-L-\alpha >0$. Then \cref{nonincreasing+error} further implies that
	\begin{align}
	\Ebb[F(\yb_{k+1})]\le
	\Ebb[F(\xb^{m}_k)]\le \Ebb[F(\yb_k)]+\sum\limits^{m-1}_{t=0}(L-\tfrac{1}{2\eta}+\alpha)\Ebb\left[\|\bar{\xb}_k^{t+1}-{\xb}_k^t\|^2\right].
	\end{align}
	That is, we have $\Ebb[F(\yb_k)] \le \Ebb[F(\yb_{k-1})]\le \ldots \le F(\yb_{0})$, and hence $\Ebb[F(\yb_k)] \downarrow F^*$.
		We can further upper bound \cref{c1+error} as
	\begin{align}\label{m1+error}
	\Ebb[F(\xb_k^{m})] \le & \Ebb\left[F(\bar{\xb}_k^1)+c_1\|\bar{\xb}^1_k-\xb_k^0\|^2+\sum\limits_{t=1}^{m-1}\left(L-\tfrac{1}{2\eta}\right)\|\bar{\xb}_k^{t+1}-{\xb}_k^t\|^2+\sum\limits_{t=1}^{m-1} 3\epsilon_k^t\right]\nonumber\\
	\le & E\left[F(\bar{\xb}_k^1)+c_1\|\bar{\xb}^1_k-\xb_k^0\|^2-\left(L-\tfrac{1}{2\eta}\right)\|\bar{\xb}^1_k-\xb_k^0\|^2+\sum\limits_{t=0}^{m-1}\left(L-\tfrac{1}{2\eta}\right)\|\bar{\xb}_k^{t+1}-{\xb}_k^t\|^2+\sum\limits_{t=0}^{m-1} 3\epsilon_k^t\right]\nonumber\\
	\le & \Ebb\left[F(\bar{\xb}_k^1)+\left( c_1+\tfrac{1}{2\eta}\right) \|\bar{\xb}^1_k-\xb_k^0\|^2+\sum\limits_{t=0}^{m-1}\left(L-\tfrac{1}{2\eta}+\alpha\right)\|\bar{\xb}_k^{t+1}-{\xb}_k^t\|^2\right]\nonumber\\
	\le & \Ebb\left[ F(\bar{\xb}_k^1) \right]+\Ebb\left[ \left( 2\eta L^2m+\tfrac{1}{2\eta}\right) \|\bar{\xb}^1_k-\xb_k^0\|^2 \right].
	\end{align}
	
	Define $r_k=\Ebb\left[ F(\yb_k)-F^\ast\right] $, and suppose $r_k >0$ for all $k$ (otherwise the algorithm terminates in finite steps). Applying the \KL condition with $\theta=1/2$, we obtain
	\begin{align}
	\tfrac{1}{c} (F(\xb)-F^\ast)^{\frac{1}{2}} \le \dist_{\partial F(\xb)} (\zero).
	\end{align}
	Setting $\xb=\bar{\xb}_k^1$, we obtain
	\begin{align}
	\frac{1}{c^2} (F(\bar{\xb}_k^1)-F^\ast) \le \dist_{\partial F(\bar{\xb}^1_k)}^2 (\zero) \le \left(L+\tfrac{1}{\eta}\right)^2\|\bar{\xb}^1_k-\yb_k\|^2.
	\end{align}
	Taking expectation on both sides and using the result from \cref{m1+error}, we obtain
	\begin{align}
	\frac{1}{c^2}\Ebb[F(\xb_k^m)-F^\ast]-\tfrac{2\eta L^2 m+\frac{1}{2\eta}}{c^2}\Ebb\left[\|\bar{\xb_k}^1-\xb_k^0\|^2\right] \le  \left(L+\tfrac{1}{\eta}\right)^2 \Ebb\left[\|\bar{\xb}^1_k-\yb_k\|^2\right].
	\end{align}
	Note that $\xb_k^0=\yb_k$. Then rearranging the above inequality yields
	\begin{align}
	\tfrac{1}{c^2}	\Ebb[F(\yb_{k+1})-F^\ast]	\le	\frac{1}{c^2}	E[F(\xb_k^m)-F^\ast] &\le \left[\left(L+\tfrac{1}{\eta}\right)^2+\tfrac{2\eta L^2 m+\frac{1}{2\eta}}{c^2}\right]\Ebb\left[\|\bar{\xb}^1_k-\yb_k\|^2\right]\\&\le \tfrac{\left(L+\frac{1}{\eta}\right)^2+\frac{2\eta L^2 m+\frac{1}{2\eta}}{c^2}}{\frac{1}{2\eta}-L-\alpha}\left(\Ebb[F(\yb_k)]-\Ebb[F(\yb_{k+1})]\right) ,
	\end{align}
	which can be rewritten as $r_{k+1} \le d \left(r_k-r_{k+1}\right)$
	with $d=\tfrac{c^2\left(L+\frac{1}{\eta}\right)^2+{2\eta L^2 m+\frac{1}{2\eta}}}{\frac{1}{2\eta}-L-\alpha}$.
	Then, induction yields that
	\begin{align}
	r_{k+1} \le \frac{d}{d+1}r_k \le \left(\frac{d}{d+1}\right)^{k+1}\left(F(\yb_0)-F^\ast\right).
	\end{align}
